# Supplementary material for: Self-Evolving Agents through Privileged Retrospective Distillation
Source: arXiv:2610.27495 source file (2026-10-20)
Supplement: Supplementary file 2 [file 8_appendix.tex]

\appendix
\section*{Appendix}

\section{Supplementary Implementation Details}
\label{sec:implementation}
